# Supplementary material for: CAST: Counterfactual Labels Improve Instruction Following in Vision-Language-Action Models
Source: arXiv:2508.13446 source file (2026-06-08)

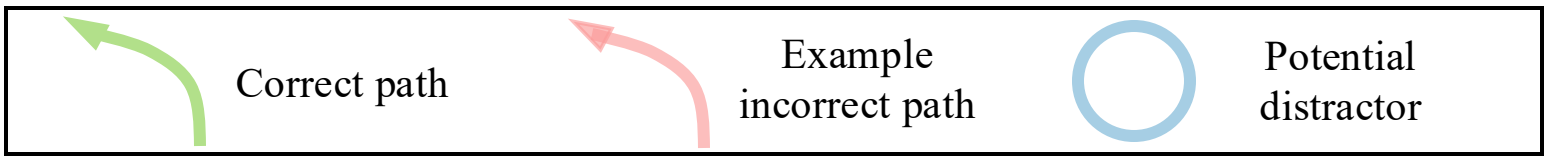

Correct path

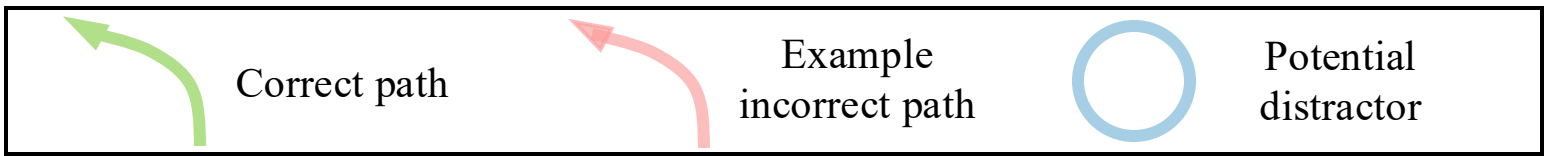

Example incorrect path

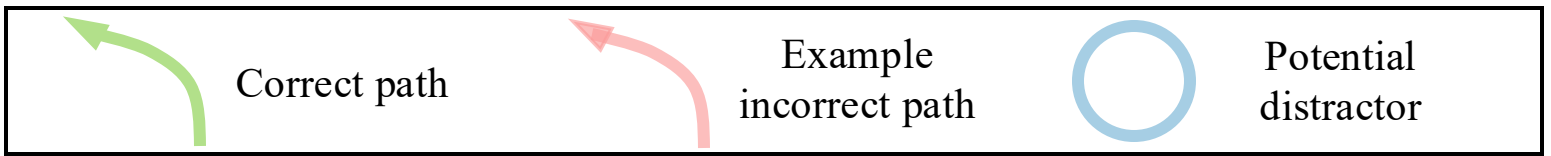

Potential distractor

Outdoor – Object Navigation

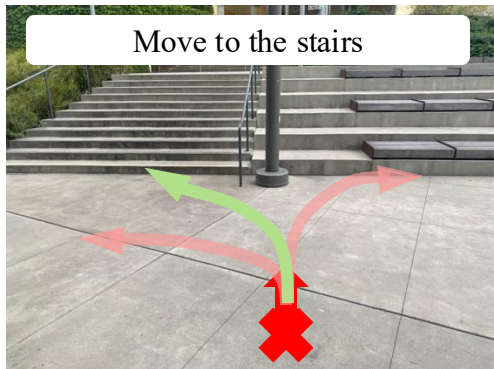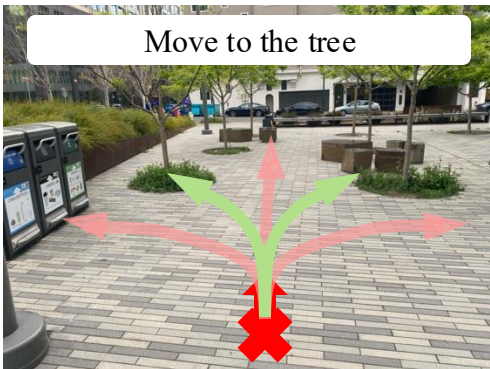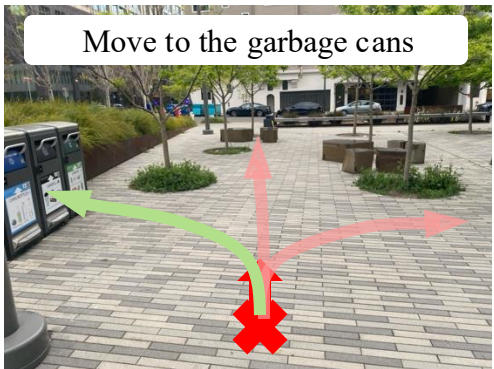

Outdoor – Continuous

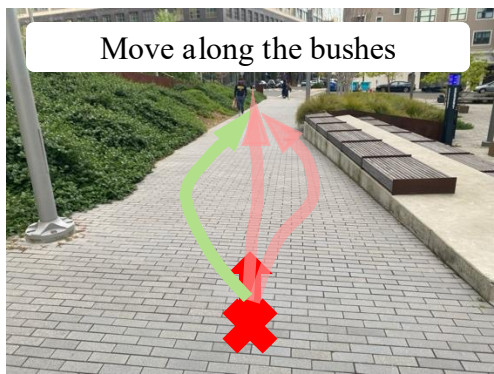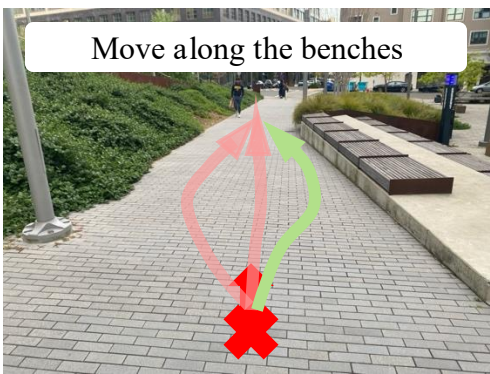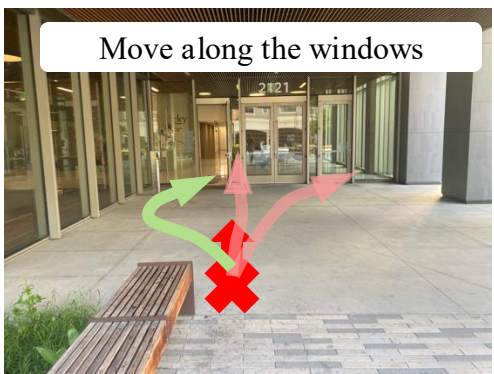

Outdoor – Referential

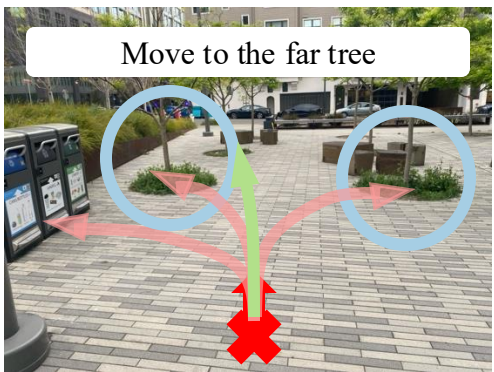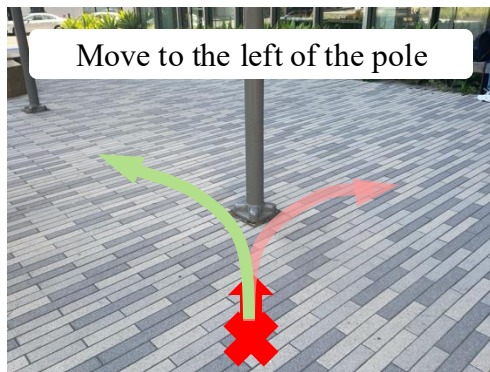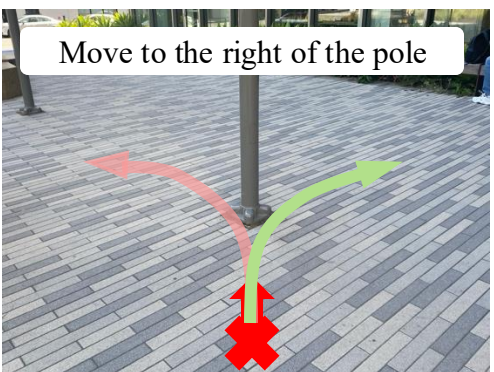

## Hallway – Object Navigation

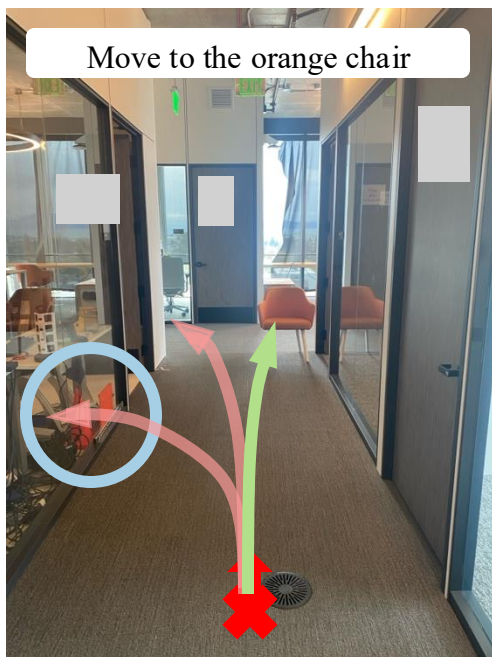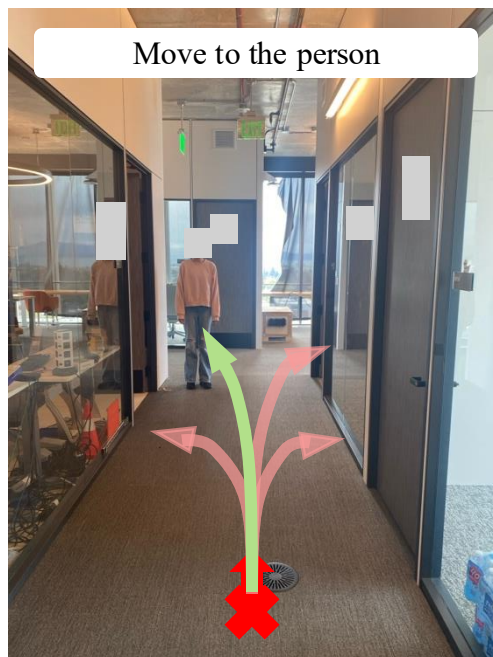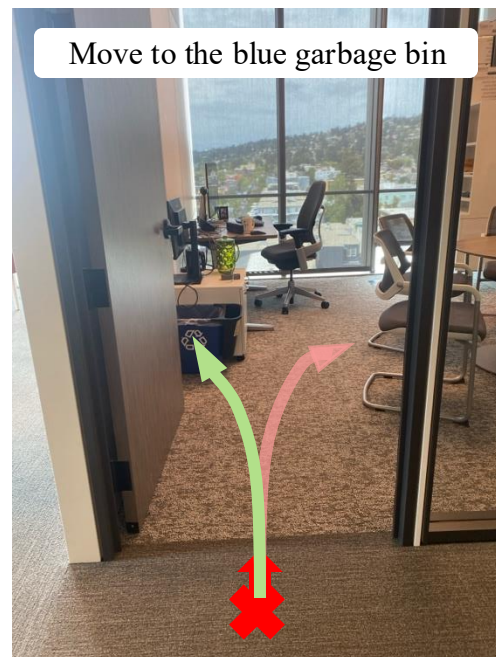

## Hallway – Continuous

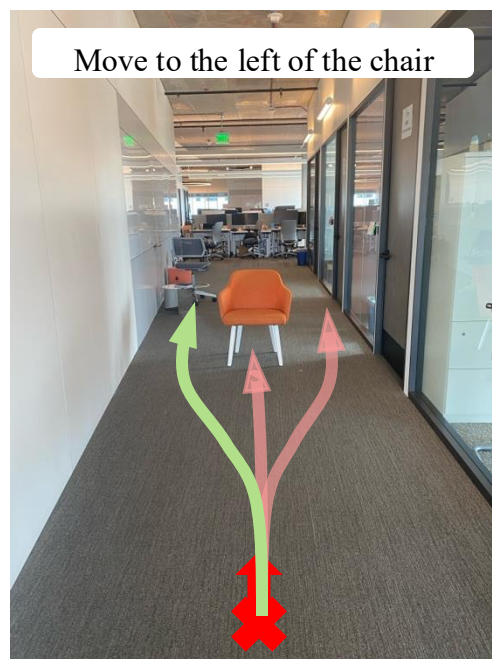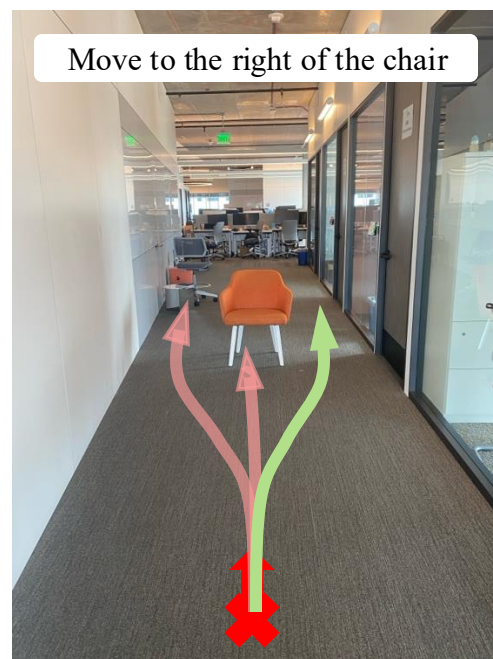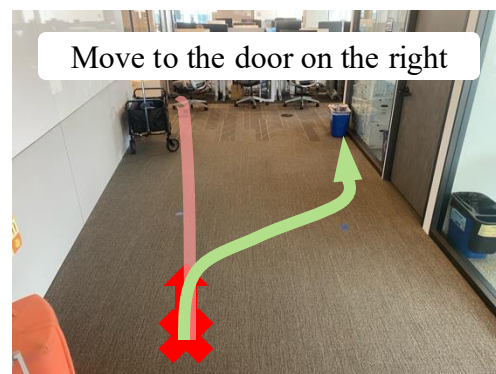

## Hallway – Referential

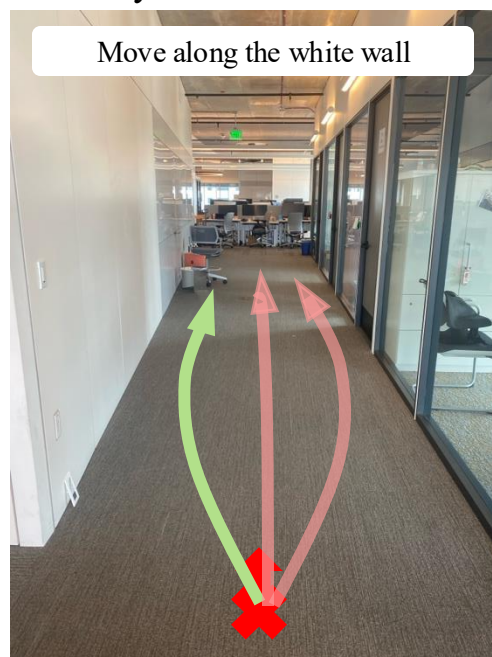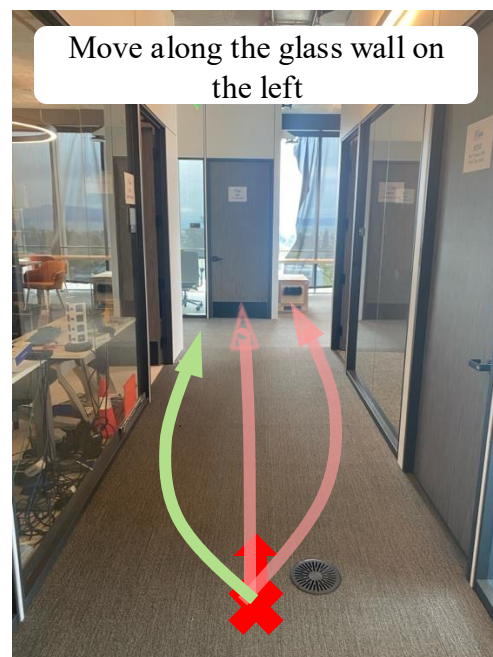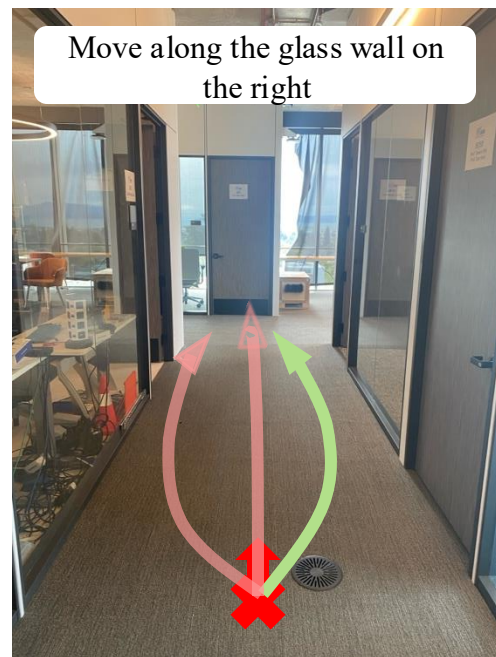

## Kitchen – Object Navigation

Move to the green garbage can

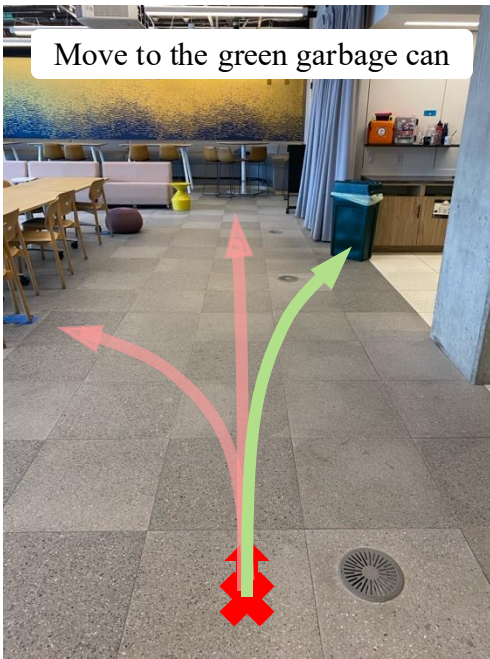

Move to the purple cushion

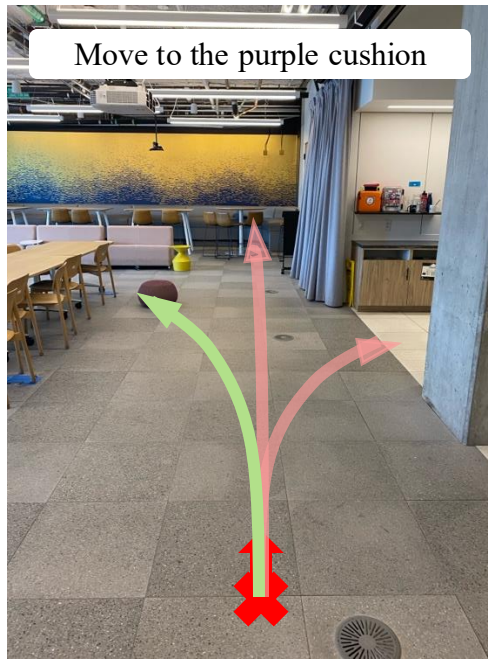

Move to the metal dishwasher

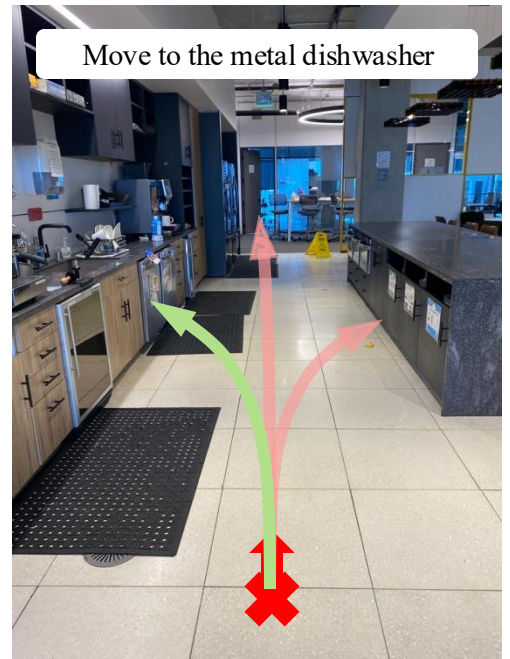

## Kitchen – Continuous

Move between the pink couch and the tables

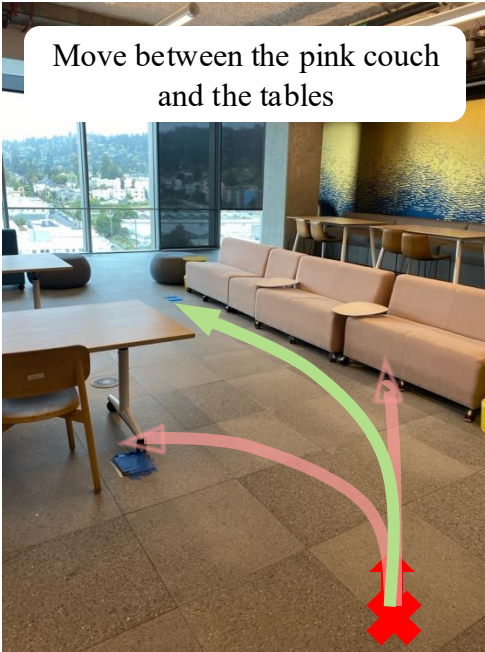

Move along the windows

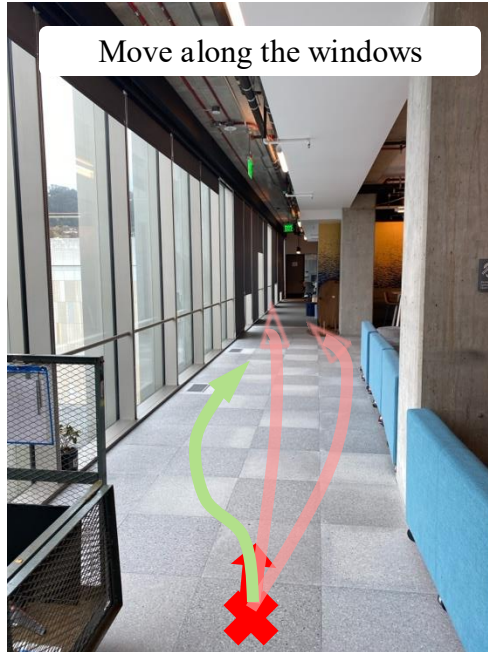

Move between the rows of chairs

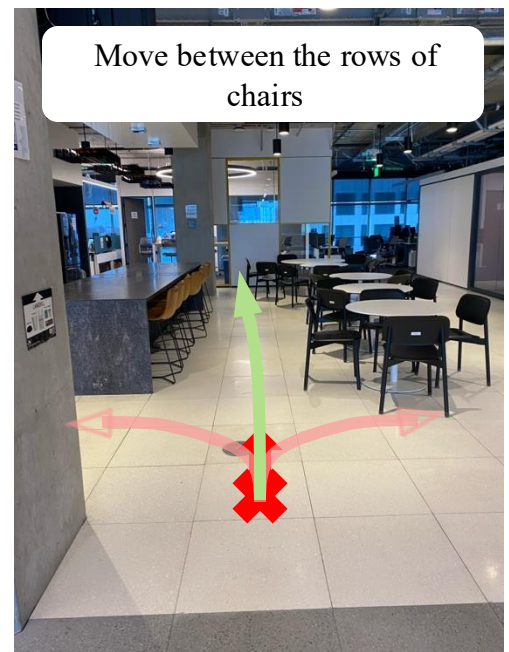

## Kitchen – Referential

Move to the left of the pillar

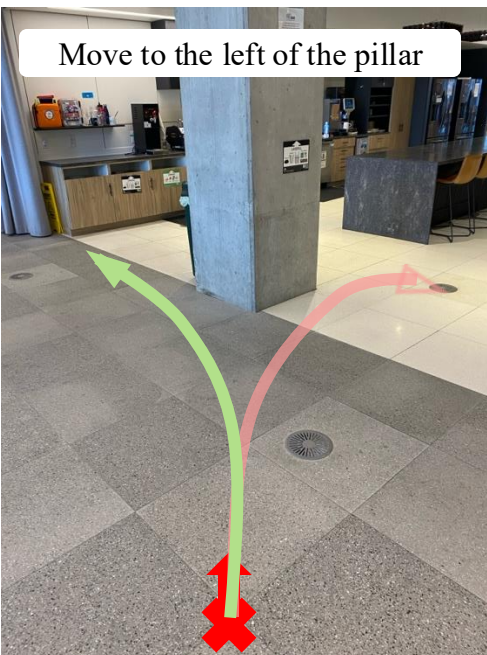

Move to the right of the pillar

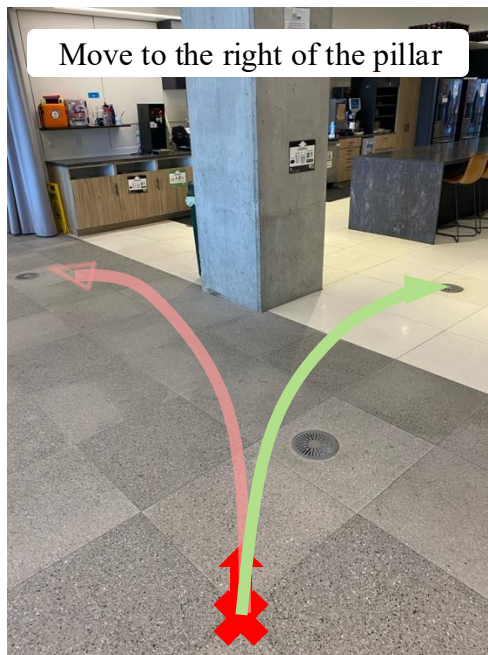

Move to the table next to the pillar

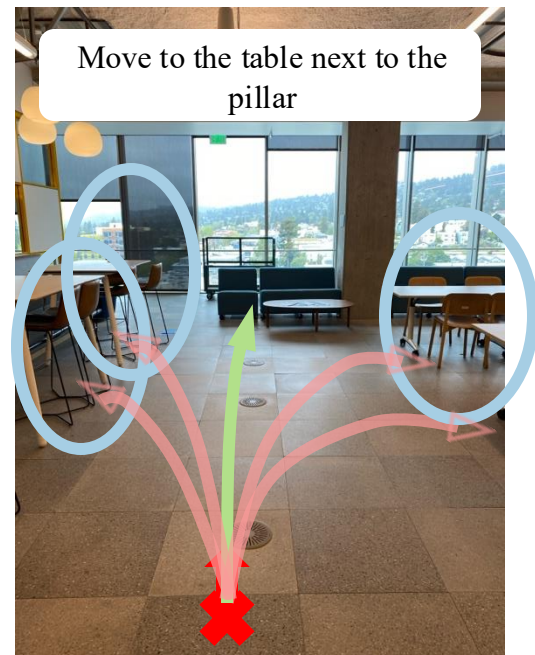

Supplement: Supplementary file 1 [file supplemental_materials.pdf]
